# Supplementary material for: Foundation Model Transparency Reports
Source: arXiv:2402.16268 source file (2024-02-26)
Supplement: Supplementary file 1 [file app_search_protocol.tex]

\hypertarget{search-protocol}{\section{Search protocol}}
\label{app:search-protocol}

In this section, we outline the search process we used to look for evidence that a foundation model developer satisfies our requirements for a given indicator. 

\subsection{General search process}

\subsubsection{Keyword Definitions}
Each item under review has associated search keywords in our GitHub repository: \url{https://github.com/stanford-crfm/fmti/}

\subsubsection{Model-Item Pair Searches}
For every model-item pair, we conduct a search using the defined keywords within the centralized resources associated with the respective models listed below.

\subsubsection{Search Methodology}
We employ the following format for every model-item-keyword tuple while using Google search, and read through the first 10 search results.

\begin{lstlisting}[breaklines=true]
site:[Refer to developer's website list below] [Refer to model name list below] [Enter keyword]
\end{lstlisting}

\noindent
For example, for GPT-4's energy efficiency item, the searches would be:

\begin{lstlisting}
site:openai.com gpt-4 energy
site:openai.com gpt-4 efficien 
\end{lstlisting}

\subsubsection{Justification}
We note the source (e.g., website, company blog post, paper) for each piece of evidence that helped confirm an item is present, alongside the justification. We link to an archive.org URL that contains the justification (instead of linking to developers’ pages directly), to maintain records.

\subsubsection{Avoid Search Personalization}
To minimize the influence of personalized search results, we perform all searches in a private or incognito browser tab.

\subsubsection{Determination Criteria}
If we find one piece of evidence that fully justifies 1 point - or, in rarer cases, 0 points - for an item, we don't perform other searches.

\subsubsection{Distribution Channels}
In certain limited cases where the above steps fail to generate any information for indicators related to distribution channels, we interact with the developer’s intended distribution channel (if disclosed), such as its API or its preferred deployment partner’s API, or the documentation related to this API. We search for the required information via this distribution channel to the extent possible. We also use proxies, such as model playgrounds, if enterprise access is otherwise required.

\subsection{Developer website}

\begin{itemize}
    \item AI21 Labs (Jurassic-2): \url{ai21.com}
    \item Amazon (Titan Text): \url{aws.amazon.com/bedrock/titan/}
    \item Anthropic (Claude): \url{anthropic.com}
    \item Cohere (Command): \url{cohere.com}
    \item Google (PaLM 2): \url{ai.google}
    \item Hugging Face (BLOOMZ): \url{bigscience.huggingface.co}
    \item Inflection (Inflection-1): \url{inflection.ai}
    \item Meta (Llama 2): \url{ai.meta.com}
    \item OpenAI (GPT-4): \url{openai.com}
    \item StabilityAI (Stable Diffusion 2): \url{stability.ai}
    
\end{itemize}

\subsection{Centralized resources for all models}

\subsubsection{AI21 Labs (Jurassic-2)}
\begin{itemize}
    \item \url{https://docs.ai21.com/docs/jurassic-2-models}
    \item \url{https://docs.ai21.com/docs/responsible-use}
    \item \url{https://uploads-ssl.webflow.com/60fd4503684b466578c0d307/61138924626a6981ee09caf6_jurassic_tech_paper.pdf}
    \item \url{https://www.ai21.com/blog/introducing-j2}
    \item \url{https://docs.ai21.com/docs/responsible-use#usage-guidelines}
    \item \url{https://studio.ai21.com/terms-of-use}
    \item \url{https://studio.ai21.com/privacy-policy}
    \item \url{https://docs.ai21.com/changelog}
\end{itemize}

\subsubsection{Amazon (Titan Text)}
\begin{itemize}
    \item \url{https://aws.amazon.com/bedrock/titan/}
    \item \url{https://docs.aws.amazon.com/pdfs/bedrock/latest/APIReference/bedrock-api.pdf#API_ListFoundationModels}
    \item \url{https://aws.amazon.com/aup/}
\end{itemize}

\subsubsection{Anthropic (Claude 2)}
\begin{itemize}
    \item \url{https://legal.anthropic.com/#aup}
    \item \url{https://vault.pactsafe.io/s/9f502c93-cb5c-4571-b205-1e479da61794/legal.html#aup}
    \item \url{https://console.anthropic.com/docs/api/supported-regions}
    \item \url{https://legal.anthropic.com/#terms}
    \item \url{https://legal.anthropic.com/#privacy}
    \item \url{https://docs.anthropic.com/claude/docs}
    \item \url{https://www.anthropic.com/index/claude-2}
    \item \url{https://www.anthropic.com/earlyaccess}
    \item \url{https://www-files.anthropic.com/production/images/Model-Card-Claude-2.pdf}
    \item \url{https://www.anthropic.com/index/frontier-threats-red-teaming-for-ai-safety}
\end{itemize}

\clearpage

\subsubsection{Cohere (Command)}
\begin{itemize}
    \item \url{https://docs.cohere.com/docs/}
    \item \url{https://cohere.com/security}
    \item \url{https://dashboard.cohere.ai/playground/generate}
    \item \url{https://cohere.com/terms-of-use}
    \item \url{https://cloud.google.com/blog/products/ai-machine-learning/accelerating-language-model-training-with-cohere-and-google-cloud-tpus}
    \item \url{https://cohere.com/data-usage-policy}
    \item \url{https://cohere.com/privacy}
    \item \url{https://cohere-inc.secureframetrust.com/}
\end{itemize}

\subsubsection{Google (PaLM 2)}
\begin{itemize}
    \item \url{https://ai.google/static/documents/palm2techreport.pdf}
    \item \url{https://developers.generativeai.google/models/language}
    \item \url{https://policies.google.com/terms/generative-ai/use-policy}
    \item \url{https://developers.generativeai.google/guide/safety_guidance}
    \item \url{https://developers.generativeai.google/products/palm}
    \item \url{https://developers.generativeai.google/available_regions}
    \item \url{https://developers.generativeai.google/terms#content_license_and_data_use}
\end{itemize}

\subsubsection{Hugging Face (BLOOMZ)}
\begin{itemize}
    \item \url{https://arxiv.org/abs/2211.01786}
    \item \url{https://huggingface.co/docs/transformers/model_doc/bloom}
    \item \url{https://huggingface.co/bigscience/bloom}
    \item \url{https://arxiv.org/abs/2303.03915}
    \item \url{https://arxiv.org/abs/2211.05100}
    \item \url{https://proceedings.neurips.cc/paper_files/paper/2022/file/ce9e92e3de2372a4b93353eb7f3dc0bd-Paper-Datasets_and_Benchmarks.pdf}
\end{itemize}

\subsubsection{Inflection (Inflection-1)}
\begin{itemize}
    \item \url{https://inflection.ai/assets/Inflection-1.pdf}
    \item \url{https://inflection.ai/inflection-1}
    \item \url{https://inflection.ai/assets/MMLU-Examples.pdf}
    \item \url{https://heypi.com/policy#privacy}
    \item \url{https://inflection.ai/safety}
\end{itemize}

\subsubsection{Meta (Llama 2)}
\begin{itemize}
    \item \url{https://arxiv.org/pdf/2307.09288.pdf}
    \item \url{https://github.com/facebookresearch/llama/blob/main/MODEL_CARD.md}
    \item \url{https://ai.meta.com/static-resource/responsible-use-guide/}
\end{itemize}

\clearpage

\subsubsection{OpenAI (GPT-4)}
\begin{itemize}
    \item \url{https://openai.com/research/gpt-4}
    \item \url{https://openai.com/policies/usage-policies}
    \item \url{https://openai.com/form/chat-model-feedback}
    \item \url{https://platform.openai.com/docs}
    \item \url{https://openai.com/customer-stories}
    \item \url{https://status.openai.com/}
    \item \url{https://openai.com/policies/terms-of-use}
    \item \url{https://cdn.openai.com/policies/employee-data-privacy-notice.pdf}
    \item \url{https://cdn.openai.com/papers/gpt-4-system-card.pdf}
    \item \url{https://arxiv.org/pdf/2303.08774.pdf}
    \item \url{https://openai.com/research/triton}
    \item \url{https://openai.com/pricing}
    \item \url{https://platform.openai.com/docs/deprecations}
    \item \url{https://openai.com/waitlist/gpt-4-api}
    \item \url{https://openai.com/our-structure}
    \item \url{https://openai.com/api-data-privacy}
\end{itemize}

\subsubsection{StabilityAI (Stable Diffusion 2)}
\begin{itemize}
    \item \url{https://huggingface.co/stabilityai/stable-diffusion-2}
    \item \url{https://openreview.net/forum?id=M3Y74vmsMcY}
    \item \url{https://huggingface.co/terms-of-service}
    \item \url{https://huggingface.co/stabilityai/stable-diffusion-2/blob/main/LICENSE-MODEL}
    \item \url{https://platform.stability.ai/legal/terms-of-service}
    \item \url{https://stability.ai/use-policy}
\end{itemize}
\clearpage
