# Supplementary material for: Foundation Model Transparency Reports
Source: arXiv:2402.16268 source file (2024-02-26)
Supplement: Supplementary file 2 [file app_transparency.tex]

\hypertarget{transparency-app}{\section{Calls for transparency}}
\label{app:transparency}

In recent years, transparency has been a rallying cry for activists, a boon to researchers, and a tangible first step for governments interested in regulating foundation models. Here we outline some of the salient calls for transparency to illustrate the different stakeholders with an interest in a more transparent foundation model ecosystem.

\textbf{Calls for transparency from governments.}

A wide variety of governments have made transparency in the development of foundation models a top priority in their wider agenda for AI regulation. 
In the U.S., the White House has secured voluntary commitments from 16 companies that include a commitment "to publicly reporting their AI systems’ capabilities, limitations, and areas of appropriate and inappropriate use" in the form of "transparency reports."\footnote{See \url{https://www.whitehouse.gov/briefing-room/statements-releases/2023/07/21/fact-sheet-biden-harris-administration-secures-voluntary-commitments-from-leading-artificial-intelligence-companies-to-manage-the-risks-posed-by-ai/} and \url{https://www.whitehouse.gov/wp-content/uploads/2023/07/Ensuring-Safe-Secure-and-Trustworthy-AI.pdf} and \url{https://www.whitehouse.gov/briefing-room/statements-releases/2023/09/12/fact-sheet-biden-harris-administration-secures-voluntary-commitments-from-eight-additional-artificial-intelligence-companies-to-manage-the-risks-posed-by-ai/} and \url{https://www.whitehouse.gov/wp-content/uploads/2023/09/Voluntary-AI-Commitments-September-2023.pdf}} 
The AI Risk Management Framework from the U.S. National Institute for Standards and Technology outlines the U.S. federal government’s current approach to transparency for foundation models and other AI systems.\footnote{\url{https://nvlpubs.nist.gov/nistpubs/ai/NIST.AI.100-1.pdf}}
The AI Risk Management Framework states "Trustworthy AI depends upon accountability. Accountability presupposes transparency. Transparency reflects the extent to which information about an AI system and its outputs is available to individuals interacting with such a system ... Meaningful transparency provides access to appropriate levels of information based on the stage of the AI lifecycle and tailored to the role or knowledge of AI actors or individuals interacting with or using the AI system." 

The SAFE framework for regulating AI proposed by Senate Majority Leader Schumer aims to ensure that "AI is developed and deployed in a responsible and transparent manner" and to "support US-led innovation in AI technologies–-including innovation in security, transparency and accountability."\footnote{\url{https://www.democrats.senate.gov/imo/media/doc/schumer_ai_framework.pdf}}
Transparency is also one of the five pillars of the bipartisan framework for a U.S. AI Act proposed by Senators Hawley and Blumenthal; their framework specifically suggests "requiring transparency from the companies developing and deploying A.I. systems" as it relates to training data, limitations, accuracy, safety, and user interaction with an AI system.\footnote{\url{https://www.blumenthal.senate.gov/imo/media/doc/09072023bipartisanaiframework.pdf}}
A variety of other draft legislation in the U.S. would require a higher level of transparency for foundation model developers, such as the Algorithmic Accountability Act\footnote{See \url{https://www.congress.gov/bill/118th-congress/house-bill/5628/all-info?s=2&r=1} and \url{https://docs.google.com/document/d/1A1bJ1mkIfE3eZuSbDmz3HGVtOvQDegHl53q3ArO7m44/}} at the federal level and California's Safety in Artificial Intelligence Act.\footnote{\url{https://leginfo.legislature.ca.gov/faces/billTextClient.xhtml?bill_id=202320240SB294}} 

%NIST https://nvlpubs.nist.gov/nistpubs/ai/NIST.AI.100-1.pdf
%AI Bill of Rights

In the EU,  transparency and information sharing have become a central focus of the draft EU AI Act. 
For instance, Article 52 of the Act imposes "transparency obligations" for some types of AI systems.
The European Parliament's draft of the AI Act included specific obligations for foundation model developers: "foundation models should have information obligations and prepare all necessary technical  documentation for potential downstream providers to be able to comply with their obligations under this Regulation. Generative foundation models should ensure transparency about the fact the content is generated by an AI system, not by humans."\footnote{\url{https://www.europarl.europa.eu/doceo/document/TA-9-2023-0236_EN.pdf}}
Developers of high-risk AI systems may also be required to provide additional transparency about their systems such that deployers have adequate information about risks and how to mitigate them.

China has gone a step further, with the central government adopting regulations that impose transparency requirements on foundation model deployers. 
China's "Interim Measures for the Management of Generative Artificial Intelligence Services" state that organizations deploying foundation models, including via an API, must "employ effective measures to increase transparency in generative AI services."\footnote{\url{http://www.cac.gov.cn/2023-07/13/c_1690898327029107.htm}} 
The law further specifies that "providers shall formulate clear, specific, and feasible tagging rules" for data and that "providers shall establish and complete mechanisms for making complaints and reports, setting up easy complaint and reporting portals, disclosing the process for handling them and the time limits for giving responses."

Many other governments have also highlighted the importance of transparency in the development and use of foundation models. 
Canada has released a "Voluntary Code of Conduct on the Responsible Development and Management of Advanced Generative AI Systems," which has been signed by Cohere, the Montreal Institute for Learning Algorithms, and the Vector Institute among other organizations.\footnote{\url{https://ised-isde.canada.ca/site/ised/en/voluntary-code-conduct-responsible-development-and-management-advanced-generative-ai-systems}} 
Canada's Voluntary Code of Conduct states that signatories commit to achieve transparency such that "sufficient information is published to allow consumers to make informed decisions and for experts to evaluate whether risks have been adequately addressed."
It further specifies that "developers of advanced generative systems available for public use" are required to "Publish information on capabilities and limitations of the system... Develop and implement a reliable and freely available method to detect content generated by the system, with a near-term focus on audio-visual content (e.g., watermarking). ... Publish a description of the types of training data used to develop the system, as well as measures taken to identify and mitigate risks." Japan is reportedly in the process of adopting its own code of conduct, which may go beyond voluntary commitments.\footnote{\url{https://english.kyodonews.net/news/2023/10/3b83adf1e28d-japans-ai-draft-guidelines-ask-for-measures-to-address-overreliance.html}}

India's report on "Impact, Opportunity, and Challenges of Generative AI," coauthored by India's Ministry of Electronics and Information Technology, states that transparency should be a central feature of India's regulatory framework for ensuring responsible use of generative AI.\footnote{\url{https://indiaai.s3.ap-south-1.amazonaws.com/docs/generative-ai-report.pdf}} The United Arab Emirates' generative AI guide, published by the Office of the Minister for Artificial Intelligence, Digital Economy, and Remote Work Applications,  highlights the importance of transparency for generative AI in terms of data protection: "Transparency is crucial to data privacy because it enables individuals to know how their data is collected, processed, and used by organizations. By being transparent, organizations can provide clear and concise information about their data privacy practices, policies, and procedures."\footnote{\url{https://ai.gov.ae/wp-content/uploads/2023/04/406.-Generative-AI-Guide_ver1-EN.pdf}} Data protection authorities around the world are "de facto regulating generative AI" by using their existing authorities, including those related to information sharing; for example, data protection authorities in Brazil, Japan, and South Korea launched investigations into OpenAI's ChatGPT in 2023.\footnote{\url{https://fpf.org/blog/how-data-protection-authorities-are-de-facto-regulating-generative-ai/}}

Some governments have highlighted the fact that existing transparency requirements already apply to foundation model developers and ought to be enforced as such.
The UK Competition and Markets Authority notes that transparency requirements are already in place under consumer protection law, and that foundation model developers must comply with the transparency provisions of the UK Consumer Rights Act.\footnote{\url{https://www.gov.uk/government/publications/ai-foundation-models-initial-report}} The U.S. Federal Trade Commission has stated that "we take note–and can take action–if companies aren’t upfront about what consumers are buying, who made it, how it was made, or what rights people have in their own creations. ... When offering a generative AI product, [companies] may need to tell customers whether and the extent to which the training data includes copyrighted or otherwise protected material."\footnote{https://www.ftc.gov/business-guidance/blog/2023/08/cant-lose-what-you-never-had-claims-about-digital-ownership-creation-age-generative-ai}

It is also worth noting that many governments have emphasized the importance of transparency in the development and use of AI systems outside of the context of foundation models. The national AI strategies of Colombia,\footnote{\url{https://colaboracion.dnp.gov.co/CDT/Conpes/Económicos/3975.pdf}}, Egypt,\footnote{\url{https://mcit.gov.eg/Upcont/Documents/Publications_672021000_Egypt-National-AI-Strategy-English.pdf}} Indonesia,\footnote{\url{https://ai-innovation.id/images/gallery/ebook/stranas-ka.pdf}}, and India\footnote{\url{https://www.niti.gov.in/sites/default/files/2019-01/NationalStrategy-for-AI-Discussion-Paper.pdf}} highlight the importance of transparency as do the national AI strategies of other countries.\footnote{\url{https://oecd.ai/en/dashboards/overview}}

\paragraph{\textbf{Calls for transparency from international organizations.}}
The UN High Commissioner for Human Rights, Volker Türk, has argued that existing rules for businesses squarely apply to foundation model developers. 
In a speech in July 2023, Türk stated that generative AI "companies must live up to their responsibilities to respect human rights in line with the Guiding Principles on Business and Human Rights."\footnote{\url{https://www.ohchr.org/en/statements/2023/07/artificial-intelligence-must-be-grounded-human-rights-says-high-commissioner}}
In addition to requiring human rights due diligence, the UN Guiding Principles on Business and Human Rights explicitly refer to transparency as it relates to a company's obligation to (i) transparently communicate the human rights impact of its products and (ii) be transparent in administering grievance processes.\footnote{For instance, the UN Guiding Principles on Business and Human Rights state, "The responsibility to respect human rights requires that business enterprises have in place policies and processes through which they can both know and show that they respect human rights in practice. Showing involves communication, providing a measure of transparency and accountability to individuals or groups who may be impacted and to other relevant stakeholders, including investors." See \url{https://www.ohchr.org/sites/default/files/documents/publications/guidingprinciplesbusinesshr_en.pdf}}

Türk further argued that without adequate guarantees of transparency, generative AI and other types of AI systems should be banned or suspended.
He said "regulations need to require assessment of the human rights risks and impacts of AI systems before, during, and after their use. Transparency guarantees, independent oversight, and access to effective remedies are needed, particularly  when the State itself is using AI technologies. AI technologies that cannot be operated in compliance with international human rights law must be  banned or suspended until such adequate safeguards are in place."

UN Secretary-General António Guterres has foregrounded transparency as well. 
The UN's digital agenda, summarized in Guterres' Global Digital Compact, makes three key proposals related to transparency: (i) the international community should "make transparency, fairness and accountability the core of AI governance," (ii) governments should "consider the adoption of a declaration on data rights that enshrines transparency," and (iii) researchers and companies should be responsible for transparently communicating the risks of AI systems.\footnote{\url{https://indonesia.un.org/sites/default/files/2023-07/our-common-agenda-policy-brief-gobal-digi-compact-en.pdf}}

The G7 Hiroshima AI Process, which was launched in May 2023 and focuses on generative AI, makes "promotion of transparency" one of its core aims.\footnote{\url{https://www.whitehouse.gov/briefing-room/statements-releases/2023/05/20/g7-hiroshima-leaders-communique/}} A September 2023 joint statement on the Hiroshima AI Process by G7 Digital and Technology Ministers committed the G7 to "develop guiding principles for organizations developing, deploying, and using advanced AI systems, in particular foundation models and generative AI," and stated that one such guiding principle could be "publicly report models’ capabilities, limitations and domains of appropriate and inappropriate use, ensuring sufficient transparency."\footnote{\url{https://www.politico.eu/wp-content/uploads/2023/09/07/3e39b82d-464d-403a-b6cb-dc0e1bdec642-230906_Ministerial-clean-Draft-Hiroshima-Ministers-Statement68.pdf}}

More broadly, international organizations have long noted that transparency is essential for responsible development of AI systems.
The OECD AI Principles, adopted in 2019, include transparency as one of five principles for trustworthy AI. 
The principle on “transparency and explainability” reads: “AI Actors should commit to transparency and responsible disclosure regarding AI systems. To this end, they should provide meaningful information, appropriate to the context, and consistent with the state of art: (i) to foster a general understanding of AI systems; (ii) to make stakeholders aware of their interactions with AI systems, including in the workplace; (iii) to enable those affected by an AI system to understand the outcome; and, (iv.) to enable those adversely affected by an AI system to challenge its outcome based on plain and easy-to-understand information on the factors, and the logic that served as the basis for the prediction, recommendation or decision.”\footnote{\url{ https://legalinstruments.oecd.org/en/instruments/OECD-LEGAL-0449}} 
The G20 AI Principles, also adopted in 2019, include this OECD principle on transparency verbatim. \footnote{\url{https://wp.oecd.ai/app/uploads/2021/06/G20-AI-Principles.pdf}} 
A number of other countries have committed to the OECD AI Principles, including Argentina, Brazil, Egypt, and Singapore.\footnote{\url{https://oecd.ai/en/ai-principles}}

\paragraph{\textbf{Calls for transparency from foundation model developers.}}

Foundation model developers have also called for greater transparency and touted the benefits of transparency in their own business practices. 
For example, in June 2022 AI21 Labs, Cohere, and OpenAI published "Joint Recommendation for Language Model Deployment" that advocated for increased transparency \citep{cohere2022}. 
Their recommendations stated that developers should “Publish usage guidelines and terms of use of LLMs ... Document known weaknesses and vulnerabilities, such as bias or ability to produce insecure code ... Documentation should also include model and use-case-specific safety best practices."

Individual developers have highlighted the importance of transparency as well. 
Anthropic ties the importance of transparency to interpretability in its paper on Constitutional AI and in describing the company's "Core Views on AI Safety" \citep{bai2022constitutional}.\footnote{As the blog post summarizing the paper states, "Constitutional AI is also helpful for transparency: we can easily specify, inspect, and understand the principles the AI system is following." See \url{https://www.anthropic.com/index/claudes-constitution and https://www.anthropic.com/index/core-views-on-ai-safety}} Inflection prioritizes transparency in its decision-making about the choices it makes with regard to safety. Inflection's Safety Policy states "Safety at its heart is a question of values. Companies choose what risks to prioritize, and how to address them. We believe the best principle is to be deliberate about these choices, and transparent with our users about the specific values we build into our AIs. We may prioritize values that you disagree with. That’s OK. We think that there is room for many perspectives ... We commit to sharing publicly what positions we aim to take in our AIs."\footnote{\url{https://inflection.ai/safety}}

OpenAI has argued that transparency can help companies work together to mitigate safety concerns regarding foundation models.\footnote{\url{https://openai.com/research/cooperation-on-safety}}
\citet{askell2019role} argue "information that companies provide about their intentions and actions—how transparent they are—can play an important role in whether other companies will cooperate with them."
OpenAI also requires transparency from its suppliers: OpenAI's Supplier Code of Conduct states that "OpenAI expects all Suppliers to adhere to the highest standards of integrity, transparency, honesty, and ethical conduct in all their business dealings."\footnote{\url{https://openai.com/policies/supplier-code}} 

Cohere states that transparency is important for its responsible development of large language models, noting that it has "invested in technical and non-technical measures to mitigate potential harm and make our development processes transparent."\footnote{\url{https://cohere.com/responsibility}} 
Cohere's Usage Guidelines prohibit users from using Cohere's platform for applications with "no transparency," meaning those that  "do not disclose that the content is generated through automated means."\footnote{\url{https://docs.cohere.com/docs/usage-guidelines}} 

Stability AI has called for transparency in connection with its advocacy for open foundation models. In a May 2023 report submitted to the U.S. Senate Judiciary Subcommittee on Privacy, Technology, and the Law, Stability AI wrote "Models like Stable Diffusion and StableLM demonstrate our commitment to AI technology that is transparent, accessible, and human-centric: ... We develop open models for transparency. Researchers can `look under the hood' to verify performance, identify potential risks, and help develop safeguards. Organizations across the public and private sector can customize these models for their own needs without exposing sensitive data or ceding control of their AI capabilities."\footnote{\url{https://stability.ai/blog/stability-ai-letter-us-senate-ai-oversight}} The report further argues "These principles can help to advance important policy objectives. Transparent models promote safety and security. ... open models enable the transparent identification, assessment, and management of risks consistent with the National Institute of Standards and Technology AI Risk Management Framework."

Hugging Face has also called for transparency as part of its push for open foundation models. In written testimony before the U.S. House Committee on Science, Space, and Technology, Hugging Face CEO Clement Delangue stated "Rigorous documentation practices for AI systems, with transparent reporting that follows well-defined protocols, serves three main goals: incentivizing responsible development; ensuring researchers and developers consider values and priorities that may otherwise be overlooked; and creating a paper trail for review. ... transparency from entities about how and where they deploy AI systems to understand what evaluations are most urgently needed."\footnote{\url{https://republicans-science.house.gov/_cache/files/5/5/551f066b-4483-4efd-b960-b36bc02d4b66/B82DBAFFA56F31799E058FB2755C2348.2023-06-22-mr.-delangue-testimony.pdf}} Hugging Face has, along with various partners, released a number of artifacts that advance transparency such as tools for exploring datasets \citep{piktus2023roots}. 

In articulating Meta's position with respect to Llama 2, \citet{touvron2023llama} state that "It is important to understand what is in the pretraining data both to increase transparency and to shed light on root causes of potential downstream issues, such as potential biases. ... open releases promote transparency and allow more people to access AI tools, democratizing the technology and decentralizing AI expertise." Meta's Responsible Use Guide for Llama 2 encourages downstream developers to "build transparency and reporting mechanisms in user interactions ... consider ways to provide transparency to end users regarding potential risks and limitations of the system prior to or at the time of user interaction."
\footnote{\url{https://ai.meta.com/static-resource/responsible-use-guide/}} 

Amazon makes clear that transparency is important with respect to the way in which it communicates its policies to users.
Amazon Web Services' Data Privacy Center states that "Our contracts are written in plain, straightforward language to be transparent and help you understand the data privacy protections that we offer. We also provide ongoing data transparency reporting."\footnote{\url{https://aws.amazon.com/compliance/data-privacy/Privacy_at_AWS_}} 

Google highlights transparency in its AI principles, writing "For datasets and models, the consistent outcome is to create and publish detailed documentation of datasets and models in the form of structured transparency artifacts known as data and model cards (see the following section for details), which function like nutrition labels, providing information such as the provenance of the data (if a data card) and model performance when tested for fairness (if a model card)."\footnote{\url{https://ai.google/static/documents/ai-principles-2022-progress-update.pdf}} 
Google's AI principles also detail the "Transparency Artifacts" that Google researchers have built, such as Healthsheets and a Data Cards Playbook.

Microsoft has also produced such artifacts, namely in the form of "Transparency Notes," which "are intended to help you understand how our AI technology works, the choices system owners can make that influence system performance and behavior, and the importance of thinking about the whole system, including the technology, the people, and the environment."\footnote{\url{https://learn.microsoft.com/en-us/legal/cognitive-services/language-service/transparency-note}} 

A large number of developers and deployers that we do not assess have also expressed the importance of transparency \citep{jobin2019global,fjeld2020principled,wef2023presidio}. Notable among them is EleutherAI, a non-profit research group that is a leading developer of open foundation models \citep{skowron2023euaiact}. 
\citet{phang2022eleutherai} write that "EleutherAI’s approach to research goes beyond transparency: by doing research entirely in public, anyone in the world can observe and contribute at every stage," adding that such public-facing research fosters a highly collaborative, diverse, and innovative research community. 

\paragraph{\textbf{Calls for transparency from researchers, civil society, and labor.}}

While governments and companies have consistently underscored the value of transparency, less powerful actors have banded together to push public and private entities to meaningfully improve transparency along with the business practices that transparency uncovers. 

Researchers have driven much of the improvement in transparency for foundation model developers, with innovations like model cards, datasheets, and data statements leading to substantial gains \citep{mitchell2018modelcards,gebru2018datasheets,bender-friedman-2018-data}.
Some have sought to solidify these improvements in transparency by strengthening the field of algorithmic auditing \citep{costanzachock2022audit}. 
Mozilla's Open Source Audit Tooling project calls for better infrastructure to evaluate and audit AI systems ~\citep{raji2022mozilla}.
Another proposal to bolster the auditing ecosystem is for governments to conduct third-party audits of AI systems under their existing authority to protect consumers and data subjects ~\citep{miller2021radical}.

Recently, coalitions of researchers led by organizations like LAION have come together to call for greater transparency in the foundation model ecosystem \citep{laion2023transparentai}.
In recent congressional hearings, expert testimony has expressed "The Need for Transparency in Artificial Intelligence" ~\citep{gregory2023testimony}.
\citet{belli2023igf} detail the central importance of transparent foundation models from the perspective of experts across Asia, Africa, and Latin America. 
Other researchers still have argued that transparency, while necessary, is far from sufficient to regulate AI ~\citep{hartzog2023oversight}.

Data workers employed as contractors by foundation model developers have also mobilized for increased transparency \citep{gray_ghost_2019}.\footnote{Some policymakers have focused on the importance of transparency with respect to data labor. For example, in a letter to the CEOs of major foundation model developers, eight members of the U.S. Congress wrote "Tech companies also must be more transparent about the role data workers play in their AI, so that consumers can make informed choices about the products they use. Unfortunately, many companies have sidestepped these duties, and that must change. ... Please share any plans your company has to be more transparent about the role its data workers play and their working conditions." See \url{https://www.markey.senate.gov/imo/media/doc/letter_to_artificial_intelligence_companies_on_data_worker_labor_conditions_-_091323pdf1.pdf}}
For example, in July 2023 members of the African Content Moderators Union filed a petition with Kenya's parliament requesting an investigation into OpenAI, Meta, Google, and other multinational technology companies that employ content moderators in Kenya.\footnote{The African Content Moderators Union has also sued Meta, alleging that it unlawfully fired workers for their union organizing. See \url{https://techcrunch.com/2023/08/23/meta-and-moderators-agree-to-mediation/}} 
The petition states that OpenAI used a vendor, Sama, to hire the petitioners as contractors who "trained the ChatGPT algorithm," and alleges that "the contracts did not sufficiently describe the nature of the job ... we were not properly informed of the nature of the work we would be undertaking." The petition further alleges that although this data labor included "reading and viewing material that depicted sexual and graphic violence and categorizing it accordingly so that ChatGPT's artificial intelligence could learn it for the purposes of its future interactions with people ... throughout the contract of training ChatGPT we were not afforded psychosocial support."\footnote{\url{https://x.com/mercymutemi/status/1678984336996028416?s=46}}

The Partnership on AI has advocated for transparency with respect to the employment of data enrichment workers, writing "While shifting how the broader field approaches data enrichment is not a trivial task, increasing transparency regarding current practices and developing more practical guidance can move the field towards improved conditions for data enrichment workers. Greater transparency can help emphasize the central role of data enrichment workers, create the basis for a rich public dialogue of how to improve conditions for workers, and increase confidence in AI models themselves."\footnote{In addition to conducting a case study in partnership with Google DeepMind exploring how to increase transparency regarding data labor, the Partnership on AI has separately published a white paper recommending that developers increase transparency in wages and pay structure for data enrichment workers. See \url{https://partnershiponai.org/wp-content/uploads/2022/11/case-study_deepmind.pdf} and \url{http://partnershiponai.org/wp-content/uploads/2021/08/PAI-Responsible-Sourcing-of-Data-Enrichment-Services.pdf}}

Civil society groups with a range of different focus areas agree that transparency is a pressing priority for policymakers and foundation model developers.
For instance, 123 civil society organizations, including AccessNow, Algorithm Watch, and the European Center for Not-for-Profit Law, released a statement advocating for the prioritization of more serious transparency requirements in the EU AI Act.\footnote{\url{https://www.fairtrials.org/app/uploads/2022/05/Civil-society-reacts-to-EP-AI-Act-draft-report_FINAL.pdf}}
The statement advocates the inclusion of a "mandatory impact assessments are a
crucial measure to ensure foresight and accountability for potential AI-related harms," and that "information on all uses of AI systems by public authorities, regardless of
the systems’ risk level, should be made public in the EU database." 
Additionally, they call for "an obligation for providers and/or users to include
information regarding the environmental impact of AI systems," which is not a provision in the EU AI Act.
Freedom House has also warned that "AI has allowed governments to refine their online censorship" and threatens to exacerbate the decline in global internet freedom.
AI has allowed governments to enhance and refine their online censorship, and foundation models may exacerbate this trend.\footnote{\url{https://freedomhouse.org/report/freedom-net/2023/repressive-power-artificial-intelligence}}
Freedom House points to transparency requirements as a mechanism to identify and combat evolving and subtle censorship pressures.

% \footnote{See \url{https://www.fairtrials.org/app/uploads/2022/05/Civil-society-reacts-to-EP-AI-Act-draft-report_FINAL.pdf} and \url{https://freedomhouse.org/report/freedom-net/2023/repressive-power-artificial-intelligence}}  \kk{@Shayne if you have the wherewithal could you turn the first link in this footnote (the reactions to the AI Act) into a sentence that name checks the groups and has a transparency quote?}

In October 2023, the U.S. Federal Trade Commission convened a workshop on the "Creative Economy and Generative AI," where creators from across different industries demanded increased transparency. In the words of one participant, "The creative economy only works when the basic tenants of consent, credit, compensation, and transparency are followed. ... Without transparency, we can't even know the extent of how much of these companies have taken. They took our work and data to train for-profit technologies that then directly compete against us in our own markets using generative media that is meant to mimic us."\footnote{\url{https://www.ftc.gov/system/files/ftc_gov/pdf/creative-economy-and-generative-ai-transcript-october-4-2023.pdf}} 

Despite its limits, transparency is a necessary and broadly popular first step towards accountability for harm caused by AI systems \citep{kaminski_2020, bates2023socially}. In the context of the rapid rollout of extremely powerful AI systems such as foundation models, transparency is all the more urgent. Companies developing and deploying foundation models should heed the call.
