# Supplementary material for: Foundation Model Transparency Reports
Source: arXiv:2402.16268 source file (2024-02-26)
Supplement: Supplementary file 4 [file indicator_output.tex]

1. Upstream → Data → \textbf{Data size}
\vspace{-\parskip}
\begin{itemize}
	\item
	\underline{Definition}: For the data used in building the model, is the data size disclosed?
	\item
	\underline{Notes}: Data size should be reported in appropriate units (e.g. bytes, words, tokens, images, frames) and broken down by modality. Data size should be reported to a precision of one significant figure (e.g. 4 trillion tokens, 200 thousand images). No form of decomposition into data phases is required.
	\item
	\underline{References}: \citet{bender-friedman-2018-data}, \citet{gebru2021datasheets}
\end{itemize}

2. Upstream → Data → \textbf{Data sources}
\vspace{-\parskip}
\begin{itemize}
	\item
	\underline{Definition}: For all data used in building the model, are the data sources disclosed?
	\item
	\underline{Notes}: To receive this point, a meaningful decomposition of sources must be listed in an understandable way (e.g. named URLs/domains/databases/data providers). It does not suffice to say data is “sourced from the Internet" or comes from "licensed sources”.
	\item
	\underline{References}: \citet{gebru2021datasheets}, \citet{hutchinson2021towards}
\end{itemize}

3. Upstream → Data → \textbf{Data creators }
\vspace{-\parskip}
\begin{itemize}
	\item
	\underline{Definition}: For all data used in building the model, is there some characterization of the people who created the data?
	\item
	\underline{Notes}: While information about data creators may not be easily discernible for some data scraped from the web, the general sources (URLs/domains) should be listed, and, for other data that is bought, licensed, or collected, a reasonable attempt at characterizing the underlying people who provided the data is required to receive this point. The relevant properties of people can vary depending on context: for example, relevant properties could include demographic information like fraction of Black individuals contributing to the dataset, geographic information like fraction of European individuals contributing to the dataset, language information like fraction of L1 English speakers, or occupational information like the fraction of professional artists.
	\item
	\underline{References}: \citet{gebru2021datasheets}, \citet{hutchinson2021towards}
\end{itemize}

4. Upstream → Data → \textbf{Data source selection}
\vspace{-\parskip}
\begin{itemize}
	\item
	\underline{Definition}: Are the selection protocols for including and excluding data sources disclosed?
	\item
	\underline{Notes}: Selection protocols refer to procedures used to choose which datasets or subsets of datasets will be used to build a model. We will award this point even if the selection protocols are non-exhaustive.
	\item
	\underline{References}: \citet{gebru2021datasheets}, \citet{hutchinson2021towards}
\end{itemize}

\clearpage5. Upstream → Data → \textbf{Data curation}
\vspace{-\parskip}
\begin{itemize}
	\item
	\underline{Definition}: For all data sources, are the curation protocols for those data sources disclosed?
	\item
	\underline{Notes}: Curation protocols refer to steps taken to further modify data sources, such as procedures to manage, annotate, and organize data. The aims of curation might include improving the quality, relevance, and representativeness of the data. We will award this point if the developer reports that it does not perform any further curation beyond the data sources.
	\item
	\underline{References}: \citet{gebru2021datasheets}, \citet{hutchinson2021towards}
\end{itemize}

6. Upstream → Data → \textbf{Data augmentation}
\vspace{-\parskip}
\begin{itemize}
	\item
	\underline{Definition}: Are any steps the developer takes to augment its data sources disclosed?
	\item
	\underline{Notes}: Such steps might include augmenting data sources with synthetic data. We will award this point if the developer reports that it does not take any steps to augment its data.
	\item
	\underline{References}: \citet{gebru2021datasheets}, \citet{hutchinson2021towards}
\end{itemize}

7. Upstream → Data → \textbf{Harmful data filtration}
\vspace{-\parskip}
\begin{itemize}
	\item
	\underline{Definition}: If data is filtered to remove harmful content, is there a description of the associated filter?
	\item
	\underline{Notes}: Such harmful content might relate to violence or child sexual abuse material. We will award this point if the developer reports that it does not perform any harmful data filtration.
	\item
	\underline{References}: \citet{dodge2021c4}, \citet{longpre2023pretrainer}
\end{itemize}

8. Upstream → Data → \textbf{Copyrighted data}
\vspace{-\parskip}
\begin{itemize}
	\item
	\underline{Definition}: For all data used in building the model, is the associated copyright status disclosed?
	\item
	\underline{Notes}: To receive this point, the copyright status (e.g. copyrighted, public domain) must relate to some decomposition of the data. We will award this point if there is some meaningful decomposition of the data, even if the decomposition is insufficient to receive the Data Creators point or if the disclosure is not comprehensive relative to legal copyright standards.
	\item
	\underline{References}: \citet{bandy2021addressing}, \citet{genlaw2023}
\end{itemize}

\clearpage9. Upstream → Data → \textbf{Data license}
\vspace{-\parskip}
\begin{itemize}
	\item
	\underline{Definition}: For all data used in building the model, is the associated license status disclosed?
	\item
	\underline{Notes}: To receive this point, the license status must relate to some decomposition of the data. We will award this point if there is some meaningful decomposition of the data, even if the decomposition is insufficient to receive the Data Creators point.
	\item
	\underline{References}: \citet{bandy2021addressing}, \citet{genlaw2023}
\end{itemize}

10. Upstream → Data → \textbf{Personal information in data}
\vspace{-\parskip}
\begin{itemize}
	\item
	\underline{Definition}: For all data used in building the model, is the inclusion or exclusion of personal information in that data disclosed?
	\item
	\underline{Notes}: To receive this point, the disclosure of personal information must relate to some decomposition of the data. We will award this point if there is some meaningful decomposition of the data, even if the decomposition is insufficient to receive the Data Creators point. Additionally, we will award this point if the developer reports the inclusion of personal information, independent of if and how they mitigate related privacy concerns.
	\item
	\underline{References}: \citet{west2019data}, \citet{brown2022does}
\end{itemize}

11. Upstream → Data labor → \textbf{Use of human labor}
\vspace{-\parskip}
\begin{itemize}
	\item
	\underline{Definition}: Are the phases of the data pipeline where human labor is involved disclosed?
	\item
	\underline{Notes}: Phases of the data pipeline that involve human labor include activities and tasks performed by people to collect, annotate, clean, or validate data. This indicator is inclusive of all data that is created by or on behalf of the developer. We will award this point if the developer gives a reasonable best-effort description of the use of human labor in their data pipeline.
	\item
	\underline{References}: \citet{kittur2013future}, \citet{dzieza2023ai}
\end{itemize}

12. Upstream → Data labor → \textbf{Employment of data laborers}
\vspace{-\parskip}
\begin{itemize}
	\item
	\underline{Definition}: Is the organization that directly employs the people involved in data labor disclosed for each phase of the data pipeline?
	\item
	\underline{Notes}: Phases of the data pipeline that involve human labor include activities and tasks performed by people to collect, annotate, clean, or validate data. This indicator is inclusive of all data that is created by or on behalf of the developer. We will award this point if the developer provides the name of the organization that employs data laborers, even if other details about the employment relationship are not disclosed.
	\item
	\underline{References}: \citet{kittur2013future}, \citet{dzieza2023ai}
\end{itemize}

\clearpage13. Upstream → Data labor → \textbf{Geographic distribution of data laborers}
\vspace{-\parskip}
\begin{itemize}
	\item
	\underline{Definition}: Is geographic information regarding the people involved in data labor disclosed for each phase of the data pipeline?
	\item
	\underline{Notes}: This indicator is inclusive of all data that is created by or on behalf of the developer. We will award this point if the developer gives a reasonable best-effort description of the geographic distribution of labor at the country-level.
	\item
	\underline{References}: \citet{hao2023cleaning}, \citet{gray2019ghost}
\end{itemize}

14. Upstream → Data labor → \textbf{Wages}
\vspace{-\parskip}
\begin{itemize}
	\item
	\underline{Definition}: Are the wages for people who perform data labor disclosed?
	\item
	\underline{Notes}: This indicator is inclusive of data labor at all points of the model development process, such as training data annotation or red teaming data used to control the model. We will award this point if the developer reports that it does not compensate workers. For all data that is created by or on behalf of the developer, 
	\item
	\underline{References}: \citet{kittur2013future}, \citet{dzieza2023ai}
\end{itemize}

15. Upstream → Data labor → \textbf{Instructions for creating data}
\vspace{-\parskip}
\begin{itemize}
	\item
	\underline{Definition}: Are the instructions given to people who perform data labor disclosed?
	\item
	\underline{Notes}: This indicator is inclusive of all data that is created by or on behalf of the developer. We will award this point if the developer makes a reasonable best-effort attempt to disclose instructions given to people who create data used to build the model for the bulk of the data phases involving human labor.
	\item
	\underline{References}: \citet{sambasivan2021everyone}, \citet{kittur2013future}
\end{itemize}

16. Upstream → Data labor → \textbf{Labor protections}
\vspace{-\parskip}
\begin{itemize}
	\item
	\underline{Definition}: Are the labor protections for people who perform data labor disclosed?
	\item
	\underline{Notes}: This indicator is inclusive of data labor at all points of the model development process, such as training data annotation or red teaming data used to control the model. It is also inclusive of all data that is created by or on behalf of the developer. As an example, labor protections might include protocols to reduce the harm to workers' mental health stemming from exposure to violent content when annotating training data. We will award this point if the developer reports that it does not protect workers or if it does not use data laborers and therefore has no labor protections.
	\item
	\underline{References}: \citet{crawford2021atlas}, \citet{gray2019ghost}
\end{itemize}

\clearpage17. Upstream → Data labor → \textbf{Third party partners}
\vspace{-\parskip}
\begin{itemize}
	\item
	\underline{Definition}: Are the third parties who were or are involved in the development of the model disclosed?
	\item
	\underline{Notes}: This indicator is inclusive of partnerships that go beyond data labor as there may be third party partners at various stages in the model development process. We will award this point if the developer reports that it was the sole entity involved in the development of the model.
	\item
	\underline{References}: \citet{crawford2021atlas}, \citet{gray2019ghost}
\end{itemize}

18. Upstream → Data access → \textbf{Queryable external data access}
\vspace{-\parskip}
\begin{itemize}
	\item
	\underline{Definition}: Are external entities provided with queryable access to the data used to build the model?
	\item
	\underline{Notes}: We will award this point for any reasonable mechanism for providing access: direct access to the data, an interface to query the data, a developer-mediated access program where developers can inspect requests, etc. Developers may receive this point even if there are rate-limits on the number of queries permitted to an external entity and restrictions on which external entities are given access, insofar as these limits and restrictions are transparent and ensure a reasonable amount of external access. We may accept justifications for prohibiting queries of specific parts of the data.
	\item
	\underline{References}: \citet{gebru2021datasheets}, \citet{piktus2023roots}
\end{itemize}

19. Upstream → Data access → \textbf{Direct external data access}
\vspace{-\parskip}
\begin{itemize}
	\item
	\underline{Definition}: Are external entities provided with direct access to the data used to build the model?
	\item
	\underline{Notes}: We will award this point if external entities can directly access the data without any form of gating from the developer. With that said, we may award this point if the developer provides justifications for prohibiting access to specific parts of the data or to unauthorized external entities.
	\item
	\underline{References}: \citet{gebru2021datasheets}, \citet{piktus2023roots}
\end{itemize}

20. Upstream → Compute → \textbf{Compute usage}
\vspace{-\parskip}
\begin{itemize}
	\item
	\underline{Definition}: Is the compute required for building the model disclosed?
	\item
	\underline{Notes}: Compute should be reported in appropriate units, which most often will be floating point operations (FLOPS). Compute should be reported to a precision of one significant figure (e.g. 5 x $10^{25}$ FLOPS). We will award this point even if there is no decomposition of the reported compute usage into compute phases, but it should be clear whether the reported compute usage is for a single model run or includes additional runs, or hyperparameter tuning, or training other models like reward models, or other steps in the model development process that necessitate compute expenditure.
	\item
	\underline{References}: \citet{henderson2020towards}, \citet{strubell2019energy}
\end{itemize}

\clearpage21. Upstream → Compute → \textbf{Development duration}
\vspace{-\parskip}
\begin{itemize}
	\item
	\underline{Definition}: Is the amount of time required to build the model disclosed?
	\item
	\underline{Notes}: The continuous duration of time required to build the model should be reported in weeks, days, or hours to a precision of one significant figure (e.g. 3 weeks). No form of decomposition into phases of building the model is required for this indicator, but it should be clear what the duration refers to (e.g. training the model, training and subsequent evaluation and red teaming).
	\item
	\underline{References}: \citet{sevilla2022compute}, \citet{hoffmann2022training}
\end{itemize}

22. Upstream → Compute → \textbf{Compute hardware}
\vspace{-\parskip}
\begin{itemize}
	\item
	\underline{Definition}: For the primary hardware used to build the model, is the amount and type of hardware disclosed?
	\item
	\underline{Notes}: In most cases, this indicator will be satisfied by information regarding the number and type of GPUs or TPUs used to train the model. The number of hardware units should be reported to a precision of one significant figure (e.g. 800 NVIDIA H100 GPUs). We will not award this point if (i) the training hardware generally used by the developer is disclosed, but the specific hardware for the given model is not, or (ii) the training hardware is disclosed, but the amount of hardware is not. We will award this point even if information about the interconnects between hardware units is not disclosed.
	\item
	\underline{References}: \citet{sevilla2022compute}, \citet{hoffmann2022training}
\end{itemize}

23. Upstream → Compute → \textbf{Hardware owner}
\vspace{-\parskip}
\begin{itemize}
	\item
	\underline{Definition}: For the primary hardware used in building the model, is the owner of the hardware disclosed?
	\item
	\underline{Notes}: For example, the hardware owner may be the model developer in the case of a self-owned cluster, a cloud provider like Microsoft Azure, Google Cloud Platform, or Amazon Web Services, or a national supercomputer. In the event that hardware is owned by multiple sources or is highly decentralized, we will award this point if a developer makes a reasonable effort to describe the distribution of hardware owners.
	\item
	\underline{References}: \citet{sevilla2022compute}, \citet{hoffmann2022training}
\end{itemize}

24. Upstream → Compute → \textbf{Energy usage}
\vspace{-\parskip}
\begin{itemize}
	\item
	\underline{Definition}: Is the amount of energy expended in building the model disclosed?
	\item
	\underline{Notes}: Energy usage should be reported in appropriate units, which most often will be megawatt-hours (mWh). Energy usage should be reported to a precision of one significant figure (e.g. 500 mWh). No form of decomposition into compute phases is required, but it should be clear whether the reported energy usage is for a single model run or includes additional runs, or hyperparameter tuning, or training other models like reward models, or other steps in the model development process that necessitate energy usage.
	\item
	\underline{References}: \citet{lacoste2019quantifying}, \citet{patterson2021carbon}
\end{itemize}

\clearpage25. Upstream → Compute → \textbf{Carbon emissions}
\vspace{-\parskip}
\begin{itemize}
	\item
	\underline{Definition}: Is the amount of carbon emitted (associated with the energy used) in building the model disclosed?
	\item
	\underline{Notes}: Emissions should be reported in appropriate units, which most often will be tons of carbon dioxide emitted (tCO2). Emissions should be reported to a precision of one significant figure (e.g. 500 tCO2). No form of decomposition into compute phases is required, but it should be clear whether the reported emissions is for a single model run or includes additional runs, or hyperparameter tuning, or training other models like reward models, or other steps in the model development process that generate emissions.
	\item
	\underline{References}: \citet{lacoste2019quantifying}, \citet{patterson2021carbon}
\end{itemize}

26. Upstream → Compute → \textbf{Broader environmental impact}
\vspace{-\parskip}
\begin{itemize}
	\item
	\underline{Definition}: Are any broader environmental impacts from building the model besides carbon emissions disclosed?
	\item
	\underline{Notes}: While the most direct environmental impact of building a foundation model is the energy used and, therefore, the potential carbon emissions, there may be other environmental impacts. For example, these may include the use of other resources such as water for cooling data centers or metals for producing specialized hardware. We recognize that there does not exist an authoritative or consensus list of broader environmental factors. For this reason, we will award this point if there is a meaningful, though potentially incomplete, discussion of broader environmental impact.
	\item
	\underline{References}: \citet{luccioni2023counting}, \citet{strubell2019energy}
\end{itemize}

27. Upstream → Methods → \textbf{Model stages}
\vspace{-\parskip}
\begin{itemize}
	\item
	\underline{Definition}: Are all stages in the model development process disclosed?
	\item
	\underline{Notes}: Stages refer to each identifiable step that constitutes a substantive change to the model during the model building process. We recognize that different developers may use different terminology for these stages, or conceptualize the stages differently. We will award this point if there is a clear and complete description of these stages.
	\item
	\underline{References}: \citet{mitchell2019model}, \citet{chung2022scaling}
\end{itemize}

28. Upstream → Methods → \textbf{Model objectives}
\vspace{-\parskip}
\begin{itemize}
	\item
	\underline{Definition}: For all stages that are described, is there a clear description of the associated learning objectives or a clear characterization of the nature of this update to the model?
	\item
	\underline{Notes}: We recognize that different developers may use different terminology for these stages, or conceptualize the stages differently. We will award this point if there is a clear description of the update to the model related to each stage, whether that is the intent of the stage (e.g. making the model less harmful), a mechanistic characterization (e.g. minimizing a specific loss function), or an empirical assessment (e.g. evaluation results conducted before and after the stage).
	\item
	\underline{References}: \citet{mitchell2019model}, \citet{chung2022scaling}
\end{itemize}

\clearpage29. Upstream → Methods → \textbf{Core frameworks}
\vspace{-\parskip}
\begin{itemize}
	\item
	\underline{Definition}: Are the core frameworks used for model development disclosed?
	\item
	\underline{Notes}: Examples of core frameworks include Tensorflow, PyTorch, Jax, Hugging Face Transformers, Seqio, T5X, Keras, SciKit, and Triton. If there are significant internal frameworks, there should be some description of their function and/or a reasonably similar publicly-available analogue. We recognize that there does not exist an authoritative or consensus list of core frameworks. For this reason, we will award this point if there is a meaningful, though potentially incomplete, list of major frameworks for the first version of the index.
	\item
	\underline{References}: \citet{mitchell2019model}, \citet{chung2022scaling}
\end{itemize}

30. Upstream → Methods → \textbf{Additional dependencies}
\vspace{-\parskip}
\begin{itemize}
	\item
	\underline{Definition}: Are any dependencies required to build the model disclosed besides data, compute, and code?
	\item
	\underline{Notes}: For example, if the model depends on an external search engine, programmable APIs, or tools, this should be disclosed. We recognize that there is not widespread consensus regarding what constitutes key dependencies beyond the data, compute, and code. We will award this point only if developers give a reasonable best-effort description of any additional dependencies or make clear that no additional dependencies are required.
	\item
	\underline{References}: \citet{lukas2023analyzing}, \citet{kim2023propile}
\end{itemize}

31. Upstream → Data Mitigations → \textbf{Mitigations for privacy}
\vspace{-\parskip}
\begin{itemize}
	\item
	\underline{Definition}: Are any steps the developer takes to mitigate the presence of PII in the data disclosed?
	\item
	\underline{Notes}: Such steps might include identifying personal information in the training data, filtering specific datasets to remove personal information, and reducing the likelihood that models will output personal information. We will award this point if the developer reports that it does not take steps to mitigate the presence of PII in the data.
	\item
	\underline{References}: \citet{kandpal2022deduplicating}, \citet{genlaw2023}
\end{itemize}

32. Upstream → Data Mitigations → \textbf{Mitigations for copyright}
\vspace{-\parskip}
\begin{itemize}
	\item
	\underline{Definition}: Are any steps the developer takes to mitigate the presence of copyrighted information in the data disclosed?
	\item
	\underline{Notes}: Such steps might include identifying copyrighted data, filtering specific datasets to remove copyrighted data, and reducing the likelihood that models will output copyrighted information. We will award this point if the developer reports that it does take steps to mitigate the presence of copyrighted information in the data.
	\item
	\underline{References}: \citet{bandy2021addressing}, \citet{genlaw2023}
\end{itemize}

\clearpage33. Model → Model basics → \textbf{Input modality}
\vspace{-\parskip}
\begin{itemize}
	\item
	\underline{Definition}: Are the input modalities for the model disclosed?
	\item
	\underline{Notes}: Input modalities refer to the types or formats of information that the model can accept as input. Examples of input modalities include text, image, audio, video, tables, graphs.
	\item
	\underline{References}: \citet{mitchell2019model}, \citet{crisan2022interactive}
\end{itemize}

34. Model → Model basics → \textbf{Output modality}
\vspace{-\parskip}
\begin{itemize}
	\item
	\underline{Definition}: Are the output modalities for the model disclosed?
	\item
	\underline{Notes}: Output modalities refer to the types or formats of information that the model can accept as output. Examples of output modalities include text, image, audio, video, tables, graphs.
	\item
	\underline{References}: \citet{mitchell2019model}, \citet{crisan2022interactive}
\end{itemize}

35. Model → Model basics → \textbf{Model components}
\vspace{-\parskip}
\begin{itemize}
	\item
	\underline{Definition}: Are all components of the model disclosed?
	\item
	\underline{Notes}: Model components refer to distinct and identifiable parts of the model. We recognize that different developers may use different terminology for model components, or conceptualize components differently. Examples include: (i) For a text-to-image model, components could refer to a text encoder and an image encoder, which may have been trained separately. (ii) For a retrieval-augmented model, components could refer to a separate retriever module.
	\item
	\underline{References}: \citet{mitchell2019model}, \citet{crisan2022interactive}
\end{itemize}

36. Model → Model basics → \textbf{Model size}
\vspace{-\parskip}
\begin{itemize}
	\item
	\underline{Definition}: For all components of the model, is the associated model size disclosed?
	\item
	\underline{Notes}: This information should be reported in appropriate units, which generally is the number of model parameters, broken down by named component. Model size should be reported to a precision of one significant figure (e.g. 500 billion parameters for text encoder, 20 billion parameters for image encoder).
	\item
	\underline{References}: \citet{mitchell2019model}, \citet{crisan2022interactive}
\end{itemize}

\clearpage37. Model → Model basics → \textbf{Model architecture}
\vspace{-\parskip}
\begin{itemize}
	\item
	\underline{Definition}: Is the model architecture disclosed?
	\item
	\underline{Notes}: Model architecture is the overall structure and organization of a foundation model, which includes the way in which any disclosed components are integrated and how data moves through the model during training or inference. We recognize that different developers may use different terminology for model architecture, or conceptualize the architecture differently. We will award this point for any clear, though potentially incomplete, description of the model architecture.
	\item
	\underline{References}: \citet{mitchell2019model}, \citet{crisan2022interactive}
\end{itemize}

38. Model → Model basics → \textbf{Centralized model documentation}
\vspace{-\parskip}
\begin{itemize}
	\item
	\underline{Definition}: Is key information about the model included in a centralized artifact such as a model card?
	\item
	\underline{Notes}: We recognize that different developers may share this information through different types of documentation, such as a system card or several clearly interrelated documents. We will award this point for the disclosure of any such centralized artifact that provides key information typically included in a model card, though the artifact may be longer-form than a standard model card (e.g. a technical report).
	\item
	\underline{References}: \citet{mitchell2019model}, \citet{crisan2022interactive}
\end{itemize}

39. Model → Model access → \textbf{External model access protocol}
\vspace{-\parskip}
\begin{itemize}
	\item
	\underline{Definition}: Is a protocol for granting external entities access to the model disclosed?
	\item
	\underline{Notes}: A model access protocol refers to the steps, requirements, and considerations involved in granting authorized model access to external entities. We will award this point if the developer discloses key details of its protocol, including (i) where external entities can request access (e.g. via an access request form); (ii) explicit criteria for selecting external entities; and (iii) a transparent decision on whether access has been granted within a specified, reasonable period of time.
	\item
	\underline{References}: \citet{solaiman2023gradient}, \citet{shevlane2022structured}
\end{itemize}

40. Model → Model access → \textbf{Blackbox external model access}
\vspace{-\parskip}
\begin{itemize}
	\item
	\underline{Definition}: Is black box model access provided to external entities?
	\item
	\underline{Notes}: Black box model access refers to the ability to query the model with inputs and receive outputs, potentially without further access. Examples of external entities that might be granted access include researchers, third-party auditors, and regulators. We will award this point for any reasonable access level: direct access to the model weights, an interface to query the model, a developer-mediated access program where developers can inspect requests, etc. Developers may receive this point even if there are rate-limits on the number of queries permitted to an external entity and restrictions on the external entities that are permitted access, insofar as these limits and restrictions are transparent.
	\item
	\underline{References}: \citet{solaiman2023gradient}, \citet{shevlane2022structured}
\end{itemize}

\clearpage41. Model → Model access → \textbf{Full external model access}
\vspace{-\parskip}
\begin{itemize}
	\item
	\underline{Definition}: Is full model access provided to external entities?
	\item
	\underline{Notes}: Full model access refers to the ability to access the model via the release of model weights. Developers may receive this point even if there are some restrictions on the external entities that are permitted access (e.g. geographic restrictions), insofar as these restrictions are transparent (e.g. via some high-level description of who has been granted access to the foundation model).
	\item
	\underline{References}: \citet{solaiman2023gradient}, \citet{shevlane2022structured}
\end{itemize}

42. Model → Capabilities → \textbf{Capabilities description}
\vspace{-\parskip}
\begin{itemize}
	\item
	\underline{Definition}: Are the model's capabilities described?
	\item
	\underline{Notes}: Capabilities refer to the specific and distinctive functions that the model can perform. We recognize that different developers may use different terminology for capabilities, or conceptualize capabilities differently. We will award this point for any clear, but potentially incomplete, description of the multiple capabilities.
	\item
	\underline{References}: \citet{srivastava2022bigbench}, \citet{liang2022helm}
\end{itemize}

43. Model → Capabilities → \textbf{Capabilities demonstration}
\vspace{-\parskip}
\begin{itemize}
	\item
	\underline{Definition}: Are the model’s capabilities demonstrated?
	\item
	\underline{Notes}: Demonstrations refer to illustrative examples or other forms of showing the model's capabilities that are legible or understandable for the general public, without requiring specific technical expertise. We recognize that different developers may use different terminology for capabilities, or conceptualize capabilities differently. We will award this point for clear demonstrations of multiple capabilities.
	\item
	\underline{References}: \citet{srivastava2022bigbench}, \citet{liang2022helm}
\end{itemize}

44. Model → Capabilities → \textbf{Evaluation of capabilities}
\vspace{-\parskip}
\begin{itemize}
	\item
	\underline{Definition}: Are the model’s capabilities rigorously evaluated, with the results of these evaluations reported prior to or concurrent with the initial release of the model?
	\item
	\underline{Notes}: Rigorous evaluations refer to precise quantifications of the model's behavior in relation to its capabilities. We recognize that capabilities may not perfectly align with evaluations, and that different developers may associate capabilities with evaluations differently. We will award this point for clear evaluations of multiple capabilities. For example, this may include evaluations of world knowledge, reasoning, state tracking or other such proficiencies. Or it may include the measurement of average performance (e.g. accuracy, F1) on benchmarks for specific tasks (e.g. text summarization, image captioning). We note that evaluations on standard broad-coverage benchmarks are likely to suffice for this indicator, though they may not if the model's capabilities are presented as especially unusual such that standard evaluations will not suffice.
	\item
	\underline{References}: \citet{srivastava2022bigbench}, \citet{liang2022helm}
\end{itemize}

\clearpage45. Model → Capabilities → \textbf{External reproducibility of capabilities evaluation}
\vspace{-\parskip}
\begin{itemize}
	\item
	\underline{Definition}: Are the evaluations of the model’s capabilities reproducible by external entities?
	\item
	\underline{Notes}: For an evaluation to be reproducible by an external entity, we mean that the associated data is either (i) publicly available or (ii) described sufficiently such that a reasonable facsimile can be constructed by an external entity. In addition, the evaluation protocol should be sufficiently described such that if the evaluation is reproduced, any discrepancies with the developer's results can be resolved. We recognize that there does not exist an authoritative or consensus standard for what is required for an evaluation to be deemed externally reproducible. Evaluations on standard benchmarks are assumed to be sufficiently reproducible for the purposes of this index. We will award this point for reproducibility of multiple disclosed evaluations. In the event that an evaluation is not reproducible, a justification by the model developer for why it is not possible for the evaluation to be made reproducible may be sufficient to score this point.
	\item
	\underline{References}: \citet{kapoor2023leakage}, \citet{liang2022helm}
\end{itemize}

46. Model → Capabilities → \textbf{Third party capabilities evaluation}
\vspace{-\parskip}
\begin{itemize}
	\item
	\underline{Definition}: Are the model’s capabilities evaluated by third parties?
	\item
	\underline{Notes}: By third party, we mean entities that are significantly or fully independent of the developer. We will award this point if (i) a third party has conducted an evaluation of model capabilities, (ii) the results of this evaluation are publicly available, and (iii) these results are disclosed or referred to in the developer’s materials.
	\item
	\underline{References}: \citet{raji2022audit}, \citet{liang2022helm}
\end{itemize}

47. Model → Limitations → \textbf{Limitations description}
\vspace{-\parskip}
\begin{itemize}
	\item
	\underline{Definition}: Are the model's limitations disclosed?
	\item
	\underline{Notes}: Limitations refer to the specific and distinctive functions that the model cannot perform (e.g. the model cannot answer questions about current events as it only contains data up to a certain time cutoff, the model is not very capable when it comes to a specific application). We recognize that different developers may use different terminology for limitations, or conceptualize limitations differently. We will award this point for any clear, but potentially incomplete, description of multiple limitations.
	\item
	\underline{References}: \citet{raji2022fallacy}, \citet{liang2022helm}
\end{itemize}

48. Model → Limitations → \textbf{Limitations demonstration}
\vspace{-\parskip}
\begin{itemize}
	\item
	\underline{Definition}: Are the model’s limitations demonstrated?
	\item
	\underline{Notes}: Demonstrations refer to illustrative examples or other forms of showing the limitations that are legible or understandable for the general public, without requiring specific technical expertise. We recognize that different developers may use different terminology for limitations, or conceptualize the limitations differently. We will award this point for clear demonstrations of multiple limitations.
	\item
	\underline{References}: \citet{raji2022fallacy}, \citet{liang2022helm}
\end{itemize}

\clearpage49. Model → Limitations → \textbf{Third party evaluation of limitations}
\vspace{-\parskip}
\begin{itemize}
	\item
	\underline{Definition}: Can the model’s limitations be evaluated by third parties?
	\item
	\underline{Notes}: By third parties, we mean entities that are significantly or fully independent of the model developers. In contrast to the third party evaluation indicators for capabilities and risks, we will award this point if third party evaluations are possible even if no third party has yet conducted them. Such evaluations are possible if, for example, the model is deployed via an API (or with open weights) and there are no restrictions on evaluating limitations (e.g. in the usage policy). 
	\item
	\underline{References}: \citet{raji2022audit}, \citet{liang2022helm}
\end{itemize}

50. Model → Risks → \textbf{Risks description}
\vspace{-\parskip}
\begin{itemize}
	\item
	\underline{Definition}: Are the model's risks disclosed?
	\item
	\underline{Notes}: Risks refer to possible negative consequences or undesirable outcomes that can arise from the model's deployment and usage. This indicator requires disclosure of risks that may arise in the event of both (i) intentional (though possibly careless) use, such as bias or hallucinations and (ii) malicious use, such as fraud or disinformation. We recognize that different developers may use different terminology for risks, or conceptualize risks differently. We will award this point for any clear, but potentially incomplete, description of multiple risks.
	\item
	\underline{References}: \citet{solaiman2023evaluating}, \citet{weidinger2021ethical}
\end{itemize}

51. Model → Risks → \textbf{Risks demonstration}
\vspace{-\parskip}
\begin{itemize}
	\item
	\underline{Definition}: Are the model’s risks demonstrated?
	\item
	\underline{Notes}: Demonstrations refer to illustrative examples or other forms of showing the risks that are legible or understandable for the general public, without requiring specific technical expertise. This indicator requires demonstration of risks that may arise in the event of both (i) intentional (though possibly careless) use, such as biases or hallucinations and (ii) malicious use, such as fraud or disinformation. We recognize that different developers may use different terminology for risks, or conceptualize risks differently. We will award this point for clear demonstrations of multiple risks.
	\item
	\underline{References}: \citet{solaiman2023evaluating}, \citet{weidinger2021ethical}
\end{itemize}

52. Model → Risks → \textbf{Unintentional harm evaluation}
\vspace{-\parskip}
\begin{itemize}
	\item
	\underline{Definition}: Are the model’s risks related to unintentional harm rigorously evaluated, with the results of these evaluations reported prior to or concurrent with the initial release of the model?
	\item
	\underline{Notes}: Rigorous evaluations refer to precise quantifications of the model's behavior in relation to such risks. Unintentional harms include bias, toxicity, and issues relating to fairness. We recognize that unintended harms may not perfectly align with risk evaluations, and that different developers may associate risks with evaluations differently. We will award this point for clear evaluations of multiple such risks. We note that evaluations on standard broad-coverage benchmarks are likely to suffice for this indicator, though they may not if the model's risks related to unintentional harm are presented as especially unusual or severe.
	\item
	\underline{References}: \citet{solaiman2023evaluating}, \citet{weidinger2021ethical}
\end{itemize}

\clearpage53. Model → Risks → \textbf{External reproducibility of unintentional harm evaluation}
\vspace{-\parskip}
\begin{itemize}
	\item
	\underline{Definition}: Are the evaluations of the model’s risks related to unintentional harm reproducible by external entities?
	\item
	\underline{Notes}: For an evaluation to be reproducible by an external entity, we mean that the associated data is either (i) publicly available or (ii) described sufficiently such that a reasonable facsimile can be constructed by the external entity. In addition, the evaluation protocol should be sufficiently described such that if the evaluation is reproduced, any discrepancies with the developer's results can be resolved. We recognize that there does not exist an authoritative or consensus standard for what is required for an evaluation to be deemed externally reproducible. Evaluations on standard benchmarks are assumed to be sufficiently reproducible for the purposes of this index. We will award this point for reproducibility of multiple disclosed evaluations. In the event that an evaluation is not reproducible, a justification by the developer for why it is not possible for the evaluation to be made reproducible may suffice.
	\item
	\underline{References}: \citet{kapoor2023leakage}, \citet{weidinger2021ethical}
\end{itemize}

54. Model → Risks → \textbf{Intentional harm evaluation}
\vspace{-\parskip}
\begin{itemize}
	\item
	\underline{Definition}: Are the model’s risks related to intentional harm rigorously evaluated, with the results of these evaluations reported prior to or concurrent with the initial release of the model?.
	\item
	\underline{Notes}: Rigorous evaluations refer to precise quantifications of the model's behavior in relation to such risks. Intentional harms include fraud, disinformation, scams, cybersecurity attacks, designing weapons or pathogens, and uses of the model for illegal purposes. We recognize that unintentional harms may not perfectly align with risk evaluations, and that different developers may associate risks with evaluations differently. We will award this point for clear evaluations of multiple such risks. We note that evaluations on standard broad-coverage benchmarks are likely to suffice for this indicator, though they may not if the model's risks related to unintentional harm are presented as especially unusual or severe.
	\item
	\underline{References}: \citet{solaiman2023evaluating}, \citet{weidinger2021ethical}
\end{itemize}

55. Model → Risks → \textbf{External reproducibility of intentional harm evaluation}
\vspace{-\parskip}
\begin{itemize}
	\item
	\underline{Definition}: Are the evaluations of the model’s risks related to intentional harm reproducible by external entities?
	\item
	\underline{Notes}: For an evaluation to be reproducible by an external entity, we mean that the associated data is either (i) publicly available or (ii) described sufficiently such that a reasonable facsimile can be constructed by the external entity. In addition, the evaluation protocol should be sufficiently described such that if the evaluation is reproduced, any discrepancies with the developer's results can be resolved. We recognize that there does not exist an authoritative or consensus standard for what is required for an evaluation to be deemed externally reproducible. Evaluations on standard benchmarks are assumed to be sufficiently reproducible for the purposes of this index. We will award this point for reproducibility of multiple disclosed evaluations. In the event that an evaluation is not reproducible, a justification by the model developer for why it is not possible for the evaluation to be made reproducible may suffice.
	\item
	\underline{References}: \citet{kapoor2023leakage}, \citet{weidinger2021ethical}
\end{itemize}

\clearpage56. Model → Risks → \textbf{Third party risks evaluation}
\vspace{-\parskip}
\begin{itemize}
	\item
	\underline{Definition}: Are the model’s risks evaluated by third parties?
	\item
	\underline{Notes}: By third party, we mean entities that are significantly or fully independent of the developer. A third party risk evaluation might involve the developer allowing a third party to choose a methodology for evaluating risks that differs from that of the developer. We will award this point if (i) a third party has conducted an evaluation of model risks, (ii) the results of this evaluation are publicly available, and (iii) these results are disclosed or referred to in the developer’s materials. If the results are not made public (but are disclosed to have been conducted) and/or the results are not discoverable in the developer’s materials, we will not award this point. We may accept a justification from either the third party or the developer for why part of the evaluation is not disclosed in relation to risks.
	\item
	\underline{References}: \citet{raji2022audit}, \citet{weidinger2021ethical}
\end{itemize}

57. Model → Model Mitigations → \textbf{Mitigations description}
\vspace{-\parskip}
\begin{itemize}
	\item
	\underline{Definition}: Are the model mitigations disclosed?
	\item
	\underline{Notes}: By model mitigations, we refer to interventions implemented by the developer at the level of the model to reduce the likelihood and/or the severity of the model’s risks. We recognize that different developers may use different terminology for mitigations, or conceptualize mitigations differently. We will award this point for any clear, but potentially incomplete, description of multiple mitigations associated with the model's risks. Alternatively, we will award this point if the developer reports that it does not mitigate risk.
	\item
	\underline{References}: \citet{solaiman2023evaluating}, \citet{weidinger2021ethical}
\end{itemize}

58. Model → Model Mitigations → \textbf{Mitigations demonstration}
\vspace{-\parskip}
\begin{itemize}
	\item
	\underline{Definition}: Are the model mitigations demonstrated?
	\item
	\underline{Notes}: Demonstrations refer to illustrative examples or other forms of showing the mitigations that are legible or understandable for the general public, without requiring specific technical expertise. We recognize that different developers may use different terminology for mitigations, or conceptualize mitigations differently. We will award this point for clear demonstrations of multiple mitigations. We will also award this point if the developer reports that it does not mitigate the risks associated with the model.
	\item
	\underline{References}: \citet{solaiman2023evaluating}, \citet{weidinger2021ethical}
\end{itemize}

59. Model → Model Mitigations → \textbf{Mitigations evaluation}
\vspace{-\parskip}
\begin{itemize}
	\item
	\underline{Definition}: Are the model mitigations rigorously evaluated, with the results of these evaluations reported?
	\item
	\underline{Notes}: Rigorous evaluations refer to precise quantifications of the model's behavior in relation to the mitigations associated with its risks. We will award this point for clear evaluations of multiple mitigations.
	\item
	\underline{References}: \citet{huang2023catastrophic}, \citet{weidinger2021ethical}
\end{itemize}

\clearpage60. Model → Model Mitigations → \textbf{External reproducibility of mitigations evaluation}
\vspace{-\parskip}
\begin{itemize}
	\item
	\underline{Definition}: Are the model mitigation evaluations reproducible by external entities?
	\item
	\underline{Notes}: For an evaluation to be reproducible by an external entity, we mean that the associated data is either (i) publicly available or (ii) described sufficiently such that a reasonable facsimile can be constructed by the external entity. In addition, the evaluation protocol should be sufficiently described such that if the evaluation is reproduced, any discrepancies with the developer's results can be resolved. In the case of mitigations evaluations, this will usually involve details about a comparison to some baseline, which may be a different, unmitigated version of the model. We recognize that there does not exist an authoritative or consensus standard for what is required for an evaluation to be deemed externally reproducible. We will award this point for reproducibility of multiple disclosed evaluations. In the event that an evaluation is not reproducible, a justification by the model developer for why it is not possible for the evaluation to be made reproducible may suffice.
	\item
	\underline{References}: \citet{kapoor2023leakage}, \citet{weidinger2021ethical}
\end{itemize}

61. Model → Model Mitigations → \textbf{Third party mitigations evaluation}
\vspace{-\parskip}
\begin{itemize}
	\item
	\underline{Definition}: Can the model mitigations be evaluated by third parties?
	\item
	\underline{Notes}: By third party, we mean entities that are significantly or fully independent of the model developers. This indicator assesses whether it is possible for third parties to assess mitigations, which is not restricted to the methods the developer uses to assess mitigations. In contrast to the third party evaluation indicators for capabilities and risks, we will award this point if third party evaluations are possible even if no third party has yet conducted them.
	\item
	\underline{References}: \citet{raji2022audit}, \citet{weidinger2021ethical}
\end{itemize}

62. Model → Trustworthiness → \textbf{Trustworthiness evaluation}
\vspace{-\parskip}
\begin{itemize}
	\item
	\underline{Definition}: Is the trustworthiness of the model rigorously evaluated, with the results of these evaluations disclosed?
	\item
	\underline{Notes}: Rigorous evaluations refer to precise quantifications of the model's behavior in relation to its trustworthiness. For example, this may include evaluations of the model’s robustness or reliability, its uncertainty, calibration, or causality, or its interpretability or explainability. We recognize that trustworthiness may not perfectly align with evaluations, and that different developers may associate trustworthiness with evaluations differently. We will award this point for a clear evaluation of the trustworthiness of the model.
	\item
	\underline{References}: \citet{brundage2020toward}, \citet{wang2023decodingtrust}
\end{itemize}

\clearpage63. Model → Trustworthiness → \textbf{External reproducibility of trustworthiness evaluation}
\vspace{-\parskip}
\begin{itemize}
	\item
	\underline{Definition}: Are the trustworthiness evaluations reproducible by external entities?
	\item
	\underline{Notes}: For an evaluation to be reproducible by an external entity, we mean that the associated data is either (i) publicly available or (ii) described sufficiently such that a reasonable facsimile can be constructed by the external entity. In addition, the evaluation protocol should be sufficiently described such that if the evaluation is reproduced, any discrepancies with the developer's results can be resolved. We recognize that there does not exist an authoritative or consensus standard for what is required for an evaluation to be deemed externally reproducible. Evaluations on standard benchmarks are assumed to be sufficiently reproducible for the purposes of this index. We will award this point for reproducibility of at least one evaluation. In the event that an evaluation is not reproducible, we may accept a justification by the model developer for why it is not possible for the evaluation to be made reproducible.
	\item
	\underline{References}: \citet{kapoor2023leakage}, \citet{shneiderman2020bridging}
\end{itemize}

64. Model → Inference → \textbf{Inference duration evaluation}
\vspace{-\parskip}
\begin{itemize}
	\item
	\underline{Definition}: Is the time required for model inference disclosed for a clearly-specified task on a clearly-specified set of hardware?
	\item
	\underline{Notes}: The duration should be reported in seconds to a precision of one significant figure (e.g. 0.002 seconds). We recognize that no established standard exists for the standardized reporting of inference evaluation. Therefore, we permit the developer to specify the task and hardware setup, as long as both are disclosed. The hardware in this evaluation need not be the hardware the developer uses for inference if it in fact does any inference itself. For example, the specific task might be generating 100,000 tokens as 5,000 sequences of length 20 and the fixed set of hardware might be 8 NVIDIA A100s. The hardware in this evaluation need not be the hardware the developer uses for inference if it in fact does any inference itself.
	\item
	\underline{References}: \citet{reddi2020mlperf}, \citet{narayanan2023cheaply}
\end{itemize}

65. Model → Inference → \textbf{Inference compute evaluation}
\vspace{-\parskip}
\begin{itemize}
	\item
	\underline{Definition}: Is the compute usage for model inference disclosed for a clearly-specified task on a clearly-specified set of hardware?
	\item
	\underline{Notes}: Compute usage for inference should be reported in FLOPS to a precision of one significant figure (e.g. 5 x $10^{25}$ FLOPS). We recognize that no established standard exists for the standardized reporting of inference evaluation. Therefore, we permit the developer to specify the task and hardware setup, as long as both are clear. For example, the specific task might be generating 100k tokens as 5k sequences of length 20 and the fixed set of hardware might be 8 NVIDIA A100s. The hardware in this evaluation need not be the hardware the developer uses for inference if it in fact does any inference itself.
	\item
	\underline{References}: \citet{reddi2020mlperf}, \citet{narayanan2023cheaply}
\end{itemize}

\clearpage66. Downstream → Distribution → \textbf{Release decision-making}
\vspace{-\parskip}
\begin{itemize}
	\item
	\underline{Definition}: Is the developer’s protocol for deciding whether or not to release a model disclosed?
	\item
	\underline{Notes}: We recognize that the release of a foundation model falls along a spectrum, with many forms of partial release, and that different developers may conceptualize release differently. We will award this point for any clear protocol that discusses the decision-making process, including if the protocol is more general to the developer rather than the specific foundation model under consideration.
	\item
	\underline{References}: \citet{solaiman2023gradient}, \citet{liang2022community-norms}
\end{itemize}

67. Downstream → Distribution → \textbf{Release process}
\vspace{-\parskip}
\begin{itemize}
	\item
	\underline{Definition}: Is a description of the process of how the model was released disclosed?
	\item
	\underline{Notes}: A description of the release process might include information about who received access to the model at what stage of the release of the model. For example, a developer might conduct a staged release where it releases the model to a select group at first and subsequently makes the model more widely available. We recognize that the release of a foundation model falls along a spectrum, with many different forms of release, and that different developers may conceptualize release differently. We will award this point for any detailed discussion of the release process, including if the discussion is more general to the developer rather than the specific foundation model under consideration.
	\item
	\underline{References}: \citet{solaiman2023gradient}, \citet{liang2022community-norms}
\end{itemize}

68. Downstream → Distribution → \textbf{Distribution channels}
\vspace{-\parskip}
\begin{itemize}
	\item
	\underline{Definition}: Are all distribution channels disclosed?
	\item
	\underline{Notes}: By distribution channel, we mean any pathway by which the model is made accessible to entities beyond the developer. We recognize that distribution channels may arise without the knowledge of the model developer. For example, the weights of a model may be released through one distribution channel and then be distributed through other channels. We will award this point if the developer discloses all of the distribution channels of which it is aware.
	\item
	\underline{References}: \citet{cobbe2023supply}, \citet{widder2023thinking}
\end{itemize}

\clearpage69. Downstream → Distribution → \textbf{Products and services}
\vspace{-\parskip}
\begin{itemize}
	\item
	\underline{Definition}: Does the developer disclose whether any products and services offered by the developer are dependent on the model?
	\item
	\underline{Notes}: We recognize that a developer may provide many products and services that depend on a foundation model or internal derivatives of the model. We will award this point for a reasonable best-effort description of any ways the developer makes internal use of the model in its products or services.
	\item
	\underline{References}: \citet{cobbe2023supply}, \citet{cen2023supplychain}
\end{itemize}

70. Downstream → Distribution → \textbf{Detection of machine-generated content}
\vspace{-\parskip}
\begin{itemize}
	\item
	\underline{Definition}: Are any mechanisms for detecting content generated by this model disclosed?
	\item
	\underline{Notes}: Such a mechanism might include storing a copy of all outputs generated by the model to compare against, implementing a watermark when generating content using the model, or training a detector post-hoc to identify such content. We will award this point if any such mechanism is disclosed or if the developer reports that it has no such mechanism.
	\item
	\underline{References}: \citet{kirchenbauer2023watermark}, \citet{Kuditipudi2023RobustDW}
\end{itemize}

71. Downstream → Distribution → \textbf{Model License}
\vspace{-\parskip}
\begin{itemize}
	\item
	\underline{Definition}: Is a license for the model disclosed?
	\item
	\underline{Notes}: In the event that licenses are written more generally, it should be clear which assets they apply to. We recognize that different developers may adopt different business models and therefor have different types of model licenses. Examples of model licenses include responsible AI licenses, open-source licenses, and licenses that allow for commercial use.
	\item
	\underline{References}: \citet{Pistilli2023}, \citet{chen2023investigation}
\end{itemize}

72. Downstream → Distribution → \textbf{Terms of service}
\vspace{-\parskip}
\begin{itemize}
	\item
	\underline{Definition}: Are terms of service disclosed for each distribution channel?
	\item
	\underline{Notes}: We will award this point if there are terms-of-service that appear to apply to the bulk of the model’s distribution channels.
	\item
	\underline{References}: \citet{rakova2022termsweservewith}, \citet{liu2021identifying}
\end{itemize}

\clearpage73. Downstream → Usage policy → \textbf{Permitted and prohibited users}
\vspace{-\parskip}
\begin{itemize}
	\item
	\underline{Definition}: Is a description of who can and cannot use the model disclosed?
	\item
	\underline{Notes}: Such restrictions may relate to countries (e.g. US-only), organizations (e.g. no competitors), industries (e.g. no weapons industry users) or other relevant factors. These restrictions on users are often contained in multiple policies; we group them here for simplicity. We will awarded this point for a clear description of permitted, restricted, and prohibited users of the model.
	\item
	\underline{References}: \citet{cohere2022}, \citet{meta2023}
\end{itemize}

74. Downstream → Usage policy → \textbf{Permitted, restricted, and prohibited uses}
\vspace{-\parskip}
\begin{itemize}
	\item
	\underline{Definition}: Are permitted, restricted, and prohibited uses of the model disclosed?
	\item
	\underline{Notes}: We will award this point if at least two of the following three categories are disclosed: (i) permitted uses, (ii) restricted uses, and (iii) prohibited uses. By restricted uses, we mean uses that require a higher level of scrutiny (such as permission from or a separate contract with the developer) to be permitted. These uses are generally included in an acceptable use policy, model license, or usage policy.
	\item
	\underline{References}: \citet{cohere2022}, \citet{meta2023}
\end{itemize}

75. Downstream → Usage policy → \textbf{Usage policy enforcement}
\vspace{-\parskip}
\begin{itemize}
	\item
	\underline{Definition}: Is the enforcement protocol for the usage policy disclosed?
	\item
	\underline{Notes}: By enforcement protocol, we refer to (i) mechanisms for identifying permitted and prohibited users, (ii) mechanisms for identifying permitted/restricted/prohibited uses, (iii) steps the developer takes to enforce its policies related to such uses, and (iv) the developer’s procedures for carrying out these steps. We will award this point for a reasonable best-effort attempt to provide the bulk of this information, though one line indicating the developer reserves the right to terminate accounts is insufficient. Alternatively, we will award this point if the developer reports that it does not enforce its usage policy.
	\item
	\underline{References}: \citet{cohere2022}, \citet{meta2023}
\end{itemize}

76. Downstream → Usage policy → \textbf{Justification for enforcement action}
\vspace{-\parskip}
\begin{itemize}
	\item
	\underline{Definition}: Do users receive a justification when they are subject to an enforcement action for violating the usage policy?
	\item
	\underline{Notes}: For example, does the developer disclose a protocol for telling users which part of the usage policy they violated, when they did so, and what specifically was violative? Enforcement actions refer to measures to limit a user’s ability to use the model, such as banning a user or restricting their ability to purchase tokens. We will award this point if the developer discloses that it gives justification for enforcement actions or, alternatively, if it discloses that it does not provide justification for enforcement actions or that it does not enforce its usage policy.
	\item
	\underline{References}: \citet{cohere2022}, \citet{meta2023}
\end{itemize}

\clearpage77. Downstream → Usage policy → \textbf{Usage policy violation appeals mechanism}
\vspace{-\parskip}
\begin{itemize}
	\item
	\underline{Definition}: Is a mechanism for appealing potential usage policy violations disclosed?
	\item
	\underline{Notes}: We will award this point if the developer provides a usage policy violation appeals mechanism, regardless of whether it is provided via a user interface or distribution channel.
	\item
	\underline{References}: \citet{cohere2022}, \citet{meta2023}
\end{itemize}

78. Downstream → Model behavior policy → \textbf{Permitted, restricted, and prohibited model behaviors}
\vspace{-\parskip}
\begin{itemize}
	\item
	\underline{Definition}: Are model behaviors that are permitted, restricted, and prohibited disclosed?
	\item
	\underline{Notes}: We refer to a policy that includes this information as a model behavior policy, or a developer's policy on what the foundation model can and cannot do (e.g. such a policy may prohibit a model from generating child sexual abuse material). We recognize that different developers may adopt different business models and that some business models may make enforcement of a model behavior policy more or less feasible. We will award this point if at least two of the three categories (i.e. permitted, restricted, and prohibited model behaviors) are disclosed. Alternatively, we will award this point if the developer reports that it does not impose any restrictions on its model's behavior.
	\item
	\underline{References}: \citet{reuter2023im}, \citet{qi2023finetuning}
\end{itemize}

79. Downstream → Model behavior policy → \textbf{Model behavior policy enforcement}
\vspace{-\parskip}
\begin{itemize}
	\item
	\underline{Definition}: Is the enforcement protocol for the model behavior policy disclosed?
	\item
	\underline{Notes}: By enforcement protocol, we refer to mechanisms for identifying whether model behavior is permitted or prohibited and actions that may arise in the event the model behavior policy is violated. For example, the developer may make updates to the model in response to issues with the model’s adherence to the model behavior policy. We will award this point if there is a clear description of the enforcement protocol, or if the developer reports that it does not enforce its model behavior policy or that it has no such restrictions on the model’s behavior.
	\item
	\underline{References}: \citet{brundage2020toward}, \citet{qi2023finetuning}
\end{itemize}

80. Downstream → Model behavior policy → \textbf{Interoperability of usage and model behavior policies}
\vspace{-\parskip}
\begin{itemize}
	\item
	\underline{Definition}: Is the way that the usage policy and the model behavior policy interoperate disclosed?
	\item
	\underline{Notes}: For example, if a user attempts to use the model for a prohibited use such as spam, how does the model behavior policy apply if at all? We will also award this point if the developer reports that it does not impose any restrictions on its model's behavior in the event of usage policy violation.
	\item
	\underline{References}: \citet{reuter2023im}, \citet{qi2023finetuning}
\end{itemize}

\clearpage81. Downstream → User Interface → \textbf{User interaction with AI system}
\vspace{-\parskip}
\begin{itemize}
	\item
	\underline{Definition}: For distribution channels with user-facing interfaces, are users notified (i) that they are interacting with an AI system, (ii) of the specific foundation model they are interacting with, and (iii) that outputs are machine-generated?
	\item
	\underline{Notes}: A user-facing interface refers to the means by which the user interacts with the foundation model, including how the user can observe outputs from the foundation model and other notifications. We will award this point if, for all distribution channels with user-facing interfaces, the user is provided adequate transparency as to the foundation model being distributed and the potential presence of any model outputs.
	\item
	\underline{References}: \citet{qiaosi2023ux}, \citet{nakao2022responsible}
\end{itemize}

82. Downstream → User Interface → \textbf{Usage disclaimers}
\vspace{-\parskip}
\begin{itemize}
	\item
	\underline{Definition}: For distribution channels with user-facing interfaces, are users provided with disclaimers involving model use?
	\item
	\underline{Notes}: A user-facing interface refers to the means by which the user interacts with the foundation model, including how the user can observe outputs from the foundation model and other notifications. Usage disclaimers could include information about what constitutes a usage policy violations or how users should interpret model outputs. We will award this point if, for all distribution channels with user-facing interfaces, the user is provided with usage disclaimers.
	\item
	\underline{References}: \citet{qiaosi2023ux}, \citet{nakao2022responsible}
\end{itemize}

83. Downstream → User data protection → \textbf{User data protection policy}
\vspace{-\parskip}
\begin{itemize}
	\item
	\underline{Definition}: Are the protocols for how the developer stores, accesses, and shares user data disclosed?
	\item
	\underline{Notes}: We will also award this point if the developer reports that it has no user data protection policy.
	\item
	\underline{References}: \citet{nissenbaum2004contextual}, \citet{king2020privacy}
\end{itemize}

84. Downstream → User data protection → \textbf{Permitted and prohibited use of user data}
\vspace{-\parskip}
\begin{itemize}
	\item
	\underline{Definition}: Are permitted and prohibited uses of user data disclosed?
	\item
	\underline{Notes}: Developers use user data for a range of purposes such as building future models, updating existing models, and evaluating both existing and future models. We will award this point if a developer discloses its policy on the use of user data from interactions associated with this model, including both permitted and prohibited uses. This may span different distribution channels if multiple channels supply user data to the developer. Alternatively, we will award this point if the developer reports it does not impose any limits on its use of user data.
	\item
	\underline{References}: \citet{nissenbaum2004contextual}, \citet{king2020privacy}
\end{itemize}

\clearpage85. Downstream → User data protection → \textbf{Usage data access protocol}
\vspace{-\parskip}
\begin{itemize}
	\item
	\underline{Definition}: Is a protocol for granting external entities access to usage data disclosed?
	\item
	\underline{Notes}: Usage data refers to the data created through user interaction with the model, such as user inputs to the model and associated metadata such as the duration of the interaction. A usage data access protocol refers to the steps, requirements, and considerations involved in granting external entities access to usage data; this goes beyond stating the conditions under which related personal information may be shared with external entities. We will award this point for a clear description of the usage data access protocol or if the developer reports it does not share usage data with external entities.
	\item
	\underline{References}: \citet{lapowsky2018cambridge}, \citet{king2020privacy}
\end{itemize}

86. Downstream → Model Updates → \textbf{Versioning protocol}
\vspace{-\parskip}
\begin{itemize}
	\item
	\underline{Definition}: Is there a disclosed version and versioning protocol for the model?
	\item
	\underline{Notes}: By versioning, we mean that each instance of the model is uniquely identified and that the model is guaranteed to not change when referring to a fixed version number; alternatively, the version clearly indicating a specific instance of the model may be able to change by noting that it is the "latest" or an "unstable" version. We recognize that different developers may adopt different versioning practices that may differ from standard semantic versioning practices used elsewhere in software engineering.
	\item
	\underline{References}: \citet{chen2023chatgpts}, \citet{Lam2020}
\end{itemize}

87. Downstream → Model Updates → \textbf{Change log}
\vspace{-\parskip}
\begin{itemize}
	\item
	\underline{Definition}: Is there a disclosed change log for the model?
	\item
	\underline{Notes}: By change log, we mean a description associated with each change to the model (which should be indicated by a change in version number). We recognize that different developers may adopt different practices for change logs that may differ from practices used elsewhere in software engineering. We will award this point if the change log provides a clear description of changes that is legible to a technical audience.
	\item
	\underline{References}: \citet{chen2023chatgpts}, \citet{li2016watch}
\end{itemize}

88. Downstream → Model Updates → \textbf{Deprecation policy}
\vspace{-\parskip}
\begin{itemize}
	\item
	\underline{Definition}: Is there a disclosed deprecation policy for the developer?
	\item
	\underline{Notes}: By deprecation policy, we refer to a description of what it means for a model to be deprecated and how users should respond to the deprecation (e.g. instructions to migrate to a newer version). We will award this point for a clear disclosure of a deprecation policy or if there is no risk of deprication (e.g. if the developer openly releases model weights).
	\item
	\underline{References}: \citet{chen2023chatgpts}, \citet{haryono2020automatic}
\end{itemize}

\clearpage89. Downstream → Feedback → \textbf{Feedback mechanism}
\vspace{-\parskip}
\begin{itemize}
	\item
	\underline{Definition}: Is a feedback mechanism disclosed?
	\item
	\underline{Notes}: By feedback mechanism, we refer to a means for external entities to report feedback or issues that arise in relation to the foundation model. Such entities may include but are not necessarily limited to users. We will award this point if the developer discloses a feedback mechanism that has been implemented.
	\item
	\underline{References}: \citet{bommasani2023ecosystem}, \citet{raji2022audit}
\end{itemize}

90. Downstream → Feedback → \textbf{Feedback summary}
\vspace{-\parskip}
\begin{itemize}
	\item
	\underline{Definition}: Is a report or summary disclosed regarding the feedback the developer received or, alternatively, the way the developer responded to that feedback?
	\item
	\underline{Notes}: We recognize that there does not exist an authoritative or consensus standard for what is required in a feedback report. For this reason, we will award this point if there is a meaningful, though potentially vague or incomplete, summary of feedback received.
	\item
	\underline{References}: \citet{chen2021achieving}, \citet{piorkowski2022evaluating}
\end{itemize}

91. Downstream → Feedback → \textbf{Government inquiries}
\vspace{-\parskip}
\begin{itemize}
	\item
	\underline{Definition}: Is a summary of government inquiries related to the model received by the developer disclosed?
	\item
	\underline{Notes}: Such government inquiries might include requests for user data, requests that certain content be banned, or requests for information about a developer’s business practices. We recognize that there does not exist an authoritative or consensus standard for what is required for such a summary of government inquiries. For this reason, we will award this point if (i) there is a meaningful, though potentially vague or incomplete, summary of government inquiries, or (ii) a summary of government inquiries related to user data.
	\item
	\underline{References}: \citet{chou2012government}, \citet{bommasani2023ecosystem}
\end{itemize}

92. Downstream → Impact → \textbf{Monitoring mechanism}
\vspace{-\parskip}
\begin{itemize}
	\item
	\underline{Definition}: For each distribution channel, is a monitoring mechanism for tracking model use disclosed?
	\item
	\underline{Notes}: By monitoring mechanism, we refer to a specific protocol for tracking model use that goes beyond an acknowledgement that usage data is collected. We will also award this point for a reasonable best-effort attempt to describe monitoring mechanisms, or if a developer discloses that a distribution channel is not monitored.
	\item
	\underline{References}: \citet{springer2018progressive}, \citet{bommasani2023ecosystem}
\end{itemize}

\clearpage93. Downstream → Impact → \textbf{Downstream applications}
\vspace{-\parskip}
\begin{itemize}
	\item
	\underline{Definition}: Across all forms of downstream use, is the number of applications dependent on the foundation model disclosed?
	\item
	\underline{Notes}: We recognize that there does not exist an authoritative or consensus standard for what qualifies as an application. We will award this point if there is a meaningful estimate of the number of downstream applications, along with some description of what it means for an application to be dependent on the model.
	\item
	\underline{References}: \citet{vipra2023concentration}, \citet{bommasani2023ecosystem}
\end{itemize}

94. Downstream → Impact → \textbf{Affected market sectors}
\vspace{-\parskip}
\begin{itemize}
	\item
	\underline{Definition}: Across all downstream applications, is the fraction of applications corresponding to each market sector disclosed?
	\item
	\underline{Notes}: By market sector, we refer to an identifiable part of the economy. While established standards exist for describing market sectors, we recognize that developers may provide vague or informal characterizations of market impact. We will award this point if there is a meaningful, though potentially vague or incomplete, summary of affected market sectors.
	\item
	\underline{References}: \citet{vipra2023concentration}, \citet{bommasani2023ecosystem}
\end{itemize}

95. Downstream → Impact → \textbf{Affected individuals}
\vspace{-\parskip}
\begin{itemize}
	\item
	\underline{Definition}: Across all forms of downstream use, is the number of individuals affected by the foundation model disclosed?
	\item
	\underline{Notes}: By affected individuals, we principally mean the number of potential users of applications. We recognize that there does not exist an authoritative or consensus standard for what qualifies as an affected individual. We will award this point if there is a meaningful estimate of the number of affected individuals along with a clear description of what it means for an individual to be affected by the model.
	\item
	\underline{References}: \citet{vipra2023concentration}, \citet{bommasani2023ecosystem}
\end{itemize}

96. Downstream → Impact → \textbf{Usage reports}
\vspace{-\parskip}
\begin{itemize}
	\item
	\underline{Definition}: Is a usage report that gives usage statistics describing the impact of the model on users disclosed?
	\item
	\underline{Notes}: We recognize that there does not exist an authoritative or consensus standard for what is required in a usage report. Usage statistics might include, for example, a description of the major categories of harm that has been caused by use of the model. We will award this point if there is a meaningful, though potentially vague or incomplete, summary of usage statistics.
	\item
	\underline{References}: \citet{brown2023allocating}, \citet{bommasani2023ecosystem}
\end{itemize}

\clearpage97. Downstream → Impact → \textbf{Geographic statistics}
\vspace{-\parskip}
\begin{itemize}
	\item
	\underline{Definition}: Across all forms of downstream use, are statistics of model usage across geographies disclosed?
	\item
	\underline{Notes}: We will award this point if there is a meaningful, though potentially incomplete or vague, disclosure of geographic usage statistics at the country-level.
	\item
	\underline{References}: \citet{brown2023allocating}, \citet{bommasani2023ecosystem}
\end{itemize}

98. Downstream → Impact → \textbf{Redress mechanism}
\vspace{-\parskip}
\begin{itemize}
	\item
	\underline{Definition}: Is any mechanism to provide redress to users for harm disclosed?
	\item
	\underline{Notes}: We will also award this point if the developer reports it does not have any such redress mechanism.
	\item
	\underline{References}: \citet{vipra2023}, \citet{bommasani2023ecosystem}
\end{itemize}

99. Downstream → Documentation for Deployers → \textbf{Centralized documentation for downstream use}
\vspace{-\parskip}
\begin{itemize}
	\item
	\underline{Definition}: Is documentation for downstream use centralized in a centralized artifact?
	\item
	\underline{Notes}: Centralized documentation for downstream use refers to an artifact, or closely-linked artifacts, that consolidate relevant information for making use of or repurposing the model. Examples of these kinds of artifacts include a website with dedicated documentation information, a github repository with dedicated documentation information, and an ecosystem card. We recognize that different developers may take different approaches to centralizing information. We will award this point if there is a clearly-identified artifact(s) that contains the majority of substantive information (e.g. capabilities, limitations, risks, evaluations, distribution channels, model license, usage policies, model behavior policies, feedback and redress mechanisms, dependencies).
	\item
	\underline{References}: \citet{gebru2021datasheets}, \citet{mitchell2019model}
\end{itemize}

100. Downstream → Documentation for Deployers → \textbf{Documentation for responsible downstream use}
\vspace{-\parskip}
\begin{itemize}
	\item
	\underline{Definition}: Is documentation for responsible downstream use disclosed?
	\item
	\underline{Notes}: Such documentation might include details on how to adjust API settings to promote responsible use, descriptions of how to implement mitigations, or guidelines for responsible use. We will also award this point if the developer states that it does not provide any such documentation. For example, the developer might state that the model is offered as is and downstream developers are accountable for using the model responsibly.
	\item
	\underline{References}: \citet{bommasani2023ecosystem}, \citet{brown2023allocating}
\end{itemize}

\clearpage
